# Supplementary material for: Near Delay-Optimal Scheduling of Batch Jobs in Multi-Server Systems
Source: arXiv:2309.16880 source file (2023-09-28)
Supplement: Supplementary file 2 [file appendices_2.tex]

\section{Proofs of Theorem~1 and Corollary 3} \label{app1}
\subsection{Proof of {\large \eqref{eq_delaygap1}} in Theorem \ref{thm1}} \label{sec_app_thm1_1}
We prove \eqref{eq_delaygap1} by using the sufficient conditions in Lemma \ref{lem1} and Corollary \ref{coro1}. The proof steps are as follows:

{\bf Construction of Policy $P'$:}
We construct an {infeasible} policy $P'$. \emph{First, in policy $P'$, all servers are busy whenever the queue is not empty.} If the number of tasks is less than $m$, some tasks are replicated over multiple servers. 
\emph{Second, the task completion times of policy $P'$ are constructed as if there is no task cancellations.} Suppose that at any time $t$, server $l$ has processed a task for $\tau$ seconds, and another copy of this task is completed at time $t$ on another server. In policy $P'$, server $l$ will cancel this task and process a new task. More specifically, in policy $P'$, server $l$ will not process the new task from scratch; instead, it is assumed that the new task assigned to server $l$ has already been processed for $\tau$ seconds by time $t$ (which is infeasible),~and server $l$ will serve the task from this progress point. If two task copies are completed at the same time on two servers, they are assumed to be distinct tasks, instead of two replicated copy of the same task. 
\emph{Finally, the completed tasks of policy $P'$ are relabelled such that each completed task is from the job with the fewest remaining tasks}. (This relabeling operation might be infeasible, because the tasks from different jobs may be simultaneously processed on parallel servers.) 
By this, policy $P'$ is constructed.

Next, we prove the conditions of Lemma \ref{lem1} one by one.

\textbf{Condition 1:} \emph{Policy $P'$ is more {work-efficient} than any policy $\pi\in\Pi$}. 
%Recall that $\bm{T}(\pi)=(T_1(\pi),\ldots, T_{k_{\text{sum}}}(\pi))$ is the sequence of task completion times of the system. 
\ifreport
\begin{proof}[Proof of Condition 1]
\else
\begin{proof}[of Condition 1]
\fi
We prove condition 1 by induction. Consider the first task completion time $T_1(\pi)$. Job 1 arrives at time $a_1=0$. 
If policy $\pi$ is non-preemptive and work-conserving, then
\begin{align}
[T_1(\pi)|\mathcal{I}]=\min_{l=1,\ldots,m} X_l.\nonumber
\end{align} 
If policy $\pi$ is preemptive and work-conserving, then some  servers may cancel the current task and switch to process a new task at time $t\in[0,T_1(\pi))$, then Lemma \ref{lem_property_MNBUMNWU} tells us that
\begin{align}\label{eq_condition1_2_1}
\min_{l=1,\ldots,m} X_l \leq_{\text{st}}[T_1(\pi)|\mathcal{I}].
\end{align}
If policy $\pi$ is non-work-conserving, then \eqref{eq_condition1_2_1} still holds, because of the possibility of server idleness. Since policy $P'$ is non-preemptive and work-conserving, we can obtain that for all $\pi\in\Pi$
\begin{align}\label{eq_condition1_2}
[T_1(P')|\mathcal{I}]=\min_{l=1,\ldots,m} X_l\leq_{\text{st}}[T_1(\pi)|\mathcal{I}].
\end{align}

Next, consider the update from $T_j(\pi)$ to $T_{j+1}(\pi)$. Recall that $s_j$ is the $j$-th task arrival time of the system. If $s_{j+1}>T_j(\pi)$, the first $j$ tasks are completed before the $(j+1)$-th task arrives, hence all servers are idle during $[T_j(\pi),s_{j+1})$; otherwise, if $s_{j+1}\leq T_j(\pi)$, the servers can keep working after $T_j(\pi)$. For any work-conserving policy $\pi$, we can obtain
\begin{eqnarray}\label{eq_thm1_2}
T_{j+1}(\pi)\!=\max\{s_{j+1},T_j(\pi)\} + \!\min_{l=1,\ldots,m} R_{j,l}(\pi),
\end{eqnarray}
where $R_{j,l}(\pi)$ is the time duration for server $l$ to complete a task after time $\max\{s_{j+1},T_j(\pi)\}$.

Suppose that $s_{j+1}\leq T_j(\pi)$ and server $l$ has spent $\tau_l$ ($\tau_l\geq0$) seconds on a task by time $T_j(\pi)$. 
In policy $P'$,  the task completion times are constructed as if there is no task cancellations. Hence, the tail probability for the servers to complete a task after time $T_j(P')$ is 
\begin{align}\label{eq_thm1_7}
&\Pr\Big[\min_{l=1,\ldots,m} R_{j,l}(P')>t\Big]\nonumber\\
=& \Pr\Big[\min_{l=1,\ldots,m}(X_l-\tau_l)>t\Big|\bm{X}> \bm{\tau} \Big].
\end{align}
If $\pi$ is a non-preemptive work-conserving policy, some servers may cancel the tasks they are processing  at time $T_j(\pi)$. If the servers in $\mathcal{S}^c$ cancel the current task and switch to process a new task at time $T_j(\pi)$, then the tail probability for the servers to complete a task after time $T_j(\pi)$ is 
\begin{align}\label{eq_thm1_8}
&\Pr\Big[\min_{l=1,\ldots,m} R_{j,l}(\pi)>t\Big]\nonumber\\
=&\Pr\!\Big[\min\Big\{\min_{l\in\mathcal{S}}(X_l-\tau_l),\min_{l\in\mathcal{S}^c}X_l\Big\}\!>t \Big| \bm{X}_{\mathcal{S}}> \bm{\tau}_{\mathcal{S}}\Big].
\end{align} 
Combining \eqref{eq_thm1_7}, \eqref{eq_thm1_8}, and Lemma \ref{lem_property_MNBUMNWU}, yields 
\begin{align}\label{eq_min}
\min_{l=1,\ldots,m} R_{j,l}(P') \leq_{\text{st}} \min_{l=1,\ldots,m} R_{j,l}(\pi).
\end{align}
If $\pi$ is a preemptive work-conserving policy, then some servers may cancel the current task and switch to process a new task at a particular time $t\in[T_j(\pi),T_{j+1}(\pi))$.
In this case, we can use Lemma \ref{lem_property_MNBUMNWU} to show that \eqref{eq_min} holds. Hence, \eqref{eq_min} holds for all work-conserving policy $\pi$. 

Suppose that $s_{j+1}> T_j(\pi)$, then the servers start to process new tasks at time $s_{j+1}$. In this case, we can show that
\eqref{eq_min} also holds for all work-conserving policy $\pi$. 

Using \eqref{eq_thm1_2}, \eqref{eq_min}, and the fact that $s_j$ is uniquely determined by $\mathcal{I}$, it follows that for all work-conserving policy $\pi$
\begin{align}\label{eq_thm1_4}
[T_{j+1}(P') | \mathcal{I},  T_j(P') = t_j] \leq_{\text{st}} [T_{j+1}(\pi) | \mathcal{I},  T_j(\pi) = t_j'] \nonumber\\
\text{whenever}~ t_j \leq t_j',j=1,2,\ldots
\end{align}
If policy $\pi$ is non-work-conserving, \eqref{eq_thm1_2} becomes
\begin{eqnarray}\label{eq_thm1_2_1}
T_{j+1}(\pi)\!\geq\max\{s_{j+1},T_j(\pi)\} + \!\min_{l=1,\ldots,m} R_{j,l}(\pi),\nonumber
\end{eqnarray}
because of the possibility of server idleness. In this case, \eqref{eq_thm1_4} still holds. Hence, \eqref{eq_thm1_4} holds for all $\pi\in\Pi$.
Then, combining \eqref{eq_condition1_2}, \eqref{eq_thm1_4}, and Theorem 6.B.3 of \cite{StochasticOrderBook}, yields
\begin{align}%\label{eq_thm1_5}
[(T_1(P'),\ldots,T_j(P'))|\mathcal{I}] \leq_{\text{st}} [(T_1(\pi),\ldots,T_j(\pi))|\mathcal{I}],~\forall~\pi\in\Pi.\nonumber
\end{align}
Hence, condition 1 is proven.
\end{proof}

\textbf{Condition 2:} \emph{Each completed task of policy $P'$ belongs to the job with the fewest remaining tasks}. Condition 2 directly follows from the construction of policy $P'$.

\textbf{Condition 3:} \emph{It holds that} 
%\begin{align}
%\mathbb{E}\left[{D}_{\text{avg,FUT-NR}}\right]\leq \mathbb{E}\left[{D}_{\text{avg}}(P')| \mathcal{I}\right] \nonumber\\
%+\frac{1}{N}\sum_{h=1}^N \max_{\substack{S: |S|\leq k_i\\
%S\subseteq\{1,\ldots,m\}}}\!\!\mathbb{E}\left[\max_{l\in S} X_l\right].
%\end{align}
\begin{align}\label{eq_condition3}
[\bm{U}_{\uparrow}(\text{FUT-NR})|\mathcal{I}] \leq_{\text{st}} [\bm{C}_{\uparrow}(P')|\mathcal{I}].
\end{align}
We prove condition 3 by a \emph{sample-path ordering} technique, which is motivated by the second proof of the  optimality of SRPT in single-server queueing systems \cite{Smith78}. The generalization from \cite{Smith78} to this {sample-path ordering} technique is non-trivial and unexpected when this research started.

First, we define the system states of policies $P'$ and FUT-NR. 
\begin{definition}\label{def_state_P}
The system state of  policy $P'$ is specified by an infinite vector $\bm{\beta}=(\beta_1,\beta_2,\ldots)$ with non-negative, non-increasing components. At any time, the coordinates of $\bm{\beta}$ are interpreted as follows: $\beta_1$ is the maximum number of remaining tasks among all jobs in the queue, $\beta_2$ is the next greatest number of remaining tasks among all jobs in the queue, and so on, with duplications being explicitly repeated. If there are $l$ unfinished jobs in the system, then it holds that
\begin{eqnarray}
\beta_1\geq\beta_2\geq\ldots\geq\beta_l>0 = \beta_{l+1} =\beta_{l+2}=\ldots.\nonumber
\end{eqnarray}
\end{definition}

\begin{definition}\label{def_state}
The system state of FUT-NR is specified by a pair of infinite vectors $\bm{\alpha}=(\alpha_1,\alpha_2,\ldots)$ and $\bm{\delta}=(\delta_1,\delta_2,$ $\ldots)$ with non-negative components. At any time, the coordinates of $\bm{\alpha}$ and $\bm{\delta}$ are interpreted as follows: $\alpha_h$ is the number of unfinished tasks of the job associated to the $h$-th coordinate, and $\delta_h$ out of these $\alpha_h$ tasks are being processed on some servers. Hence, 
\begin{align}\label{eq_def_state}
\delta_h \leq \alpha_h\leq k_{\max},~\sum_{h=1}^\infty \delta_h\leq m. 
\end{align}
The coordinates of $\bm{\alpha}$ and $\bm{\delta}$ are sorted in the non-increasing order of $\alpha_h-\delta_h$, with duplications being explicitly repeated. 
%When $\alpha_h-\delta_h=\alpha_{i+1}-\delta_{i+1}$, the coordinates are sorted such that $\alpha_h\geq \alpha_{i+1}$. 
If there are $l$ unfinished jobs in the system, then there exists an integer $r$ ($0\leq r\leq l$) such that 
\begin{eqnarray}
&&\!\!\!\!\!\!\!\!\!\!\!\!\!\!\!\!\alpha_1-\delta_1\geq\ldots\geq \alpha_{r}-\delta_{r}>0= \alpha_{r+1}-\delta_{r+1}=\ldots,\\
&&\!\!\!\!\!\!\!\!\!\!\!\!\!\!\!\!\alpha_h \left\{\begin{array}{l l} >0, &\text{if}~ h\leq l;\\
  =0, &\text{if}~ h\geq l+1,\end{array}\right.~~\delta_h \left\{\begin{array}{l l} \geq0, &\text{if}~ h\leq l;\\
  =0, &\text{if}~ h\geq l+1.\end{array}\right.
  \end{eqnarray}
\end{definition}

Let $\{\bm{\beta}(t),t\geq0\}$ be the state process of policy $P'$ and $\{\bm{\alpha}(t),\bm{\delta}(t),t\geq0\}$ be the state process of FUT-NR, which are assumed to be right-continuous. One key result of the sample-path ordering technique is the following lemma:

\begin{lemma}\label{lemG4}
Suppose that $\bm{\alpha}(0^-) = \bm{\delta}(0^-)=\bm{\beta}(0^-)=\bm{0}$ and the job parameters $\mathcal{I}$ are given. For any sample path of policy $P'$, there exists a sample path of FUT-NR with the same probability density such that
\begin{eqnarray}\label{eq_lemG4}
\sum_{h=j}^\infty [\alpha_h(t)- \delta_h(t)]\leq \sum_{h=j}^\infty \beta_h(t)
\end{eqnarray}
holds for all $t\geq0$ and j = $1,2,\ldots$
\end{lemma}

The following lemmas are needed to prove Lemma \ref{lemG4}:

\begin{lemma}\label{lem_non_prmp1}
Suppose that, under policy FUT-NR, $\{\bm{\alpha}',\bm{\delta}'\}$ is obtained by completing a task on one server in the system whose state is $\{\bm{\alpha},\bm{\delta}\}$. Further, suppose that, under policy $P'$, $\bm{\beta}'$ is obtained by completing a task on one server in the system whose state is $\bm{\beta}$.
If
\begin{eqnarray}\label{eq_non_prmp_41}
\sum_{h=j}^\infty [\alpha_h - \delta_h]\leq \sum_{h=j}^\infty \beta_h, ~\forall~j=1,2,\ldots,\nonumber
\end{eqnarray}
then
\begin{eqnarray}\label{eq_non_prmp_40}
\sum_{h=j}^\infty [\alpha'_h - \delta'_h]\leq \sum_{h=j}^\infty \beta'_h, ~\forall~j=1,2,\ldots
\end{eqnarray}
\end{lemma}

\begin{proof}
The proof is similar to that of Lemma 2 in \cite{Smith78}.
If $\sum_{h=j}^\infty [\alpha'_h - \delta'_h]=0$, then the inequality \eqref{eq_non_prmp_40} follows naturally. 
If $\sum_{h=j}^\infty [\alpha'_h - \delta'_h]>0$, then there exist some tasks that have not been assigned to any server. 
In FUT-NR, a server that has just completed a task will be allocated to process an unassigned task from the job with the minimum positive $\alpha'_h - \delta'_h$. Hence,
$\sum_{h=j}^\infty [\alpha'_h - \delta'_h]=\sum_{h=j}^\infty [\alpha_h - \delta_h] - 1 \leq \sum_{h=j}^\infty \beta_h -1 \leq \sum_{h=j}^\infty \beta'_h$.
\end{proof}

\begin{lemma}\label{lem_non_prmp2}
Suppose that, under policy FUT-NR, $\{\bm{\alpha}',\bm{\delta}'\}$ is obtained by adding a job with $b$ tasks to the system whose state is $\{\bm{\alpha},\bm{\delta}\}$. Further, suppose that, under policy $P'$, $\bm{\beta}'$ is obtained by adding a job with $b$ tasks to the system whose state is $\bm{\beta}$.
If
\begin{eqnarray}
\sum_{h=j}^\infty [\alpha_h - \delta_h]\leq \sum_{h=j}^\infty \beta_h, ~\forall~j=1,2,\ldots,\nonumber
\end{eqnarray}
then
\begin{eqnarray}
\sum_{h=j}^\infty [\alpha'_h - \delta'_h]\leq \sum_{h=j}^\infty \beta'_h, ~\forall~j=1,2,\ldots\nonumber
\end{eqnarray}
\end{lemma}

\begin{proof}
The proof is similar to that of Lemma 3 in \cite{Smith78}.
Without loss of generalization, we suppose that after the job arrival, $b$ is the $l$-th coordinate of $\bm{\alpha}'$ and the $m$-th coordinate of $\bm{\beta}'$. Hence, $\alpha'_l = \beta'_m= b$. Because no server completes a task at this time instant, $\delta'_l =0$. We consider the following four cases:

{Case 1}: $l<j, m<j$. We can obtain $\sum_{h=j}^\infty [\alpha'_h - \delta'_h] = \sum_{h=j-1}^\infty [\alpha_h - \delta_h] \leq \sum_{h=j-1}^\infty \beta_h= \sum_{h=j}^\infty \beta_h'$.

{Case 2}: $l<j, m\geq j$. We have $\sum_{h=j}^\infty [\alpha'_h - \delta'_h] =\sum_{h=j-1}^\infty $ $[\alpha_h - \delta_h] \leq b + \sum_{h=j}^\infty [\alpha_h - \delta_h] \leq b + \sum_{h=j}^\infty \beta_h = \sum_{h=j}^\infty \beta_h'$.

{Case 3}: $l\geq j, m<j$. We have $\sum_{h=j}^\infty [\alpha'_h - \delta'_h] = b + \sum_{h=j}^\infty [\alpha_h - \delta_h] \leq \sum_{h=j-1}^\infty [\alpha_h - \delta_h] \leq \sum_{h=j-1}^\infty \beta_h = \sum_{h=j}^\infty \beta_h'$.

{Case 4}: $l\geq j, m\geq j$. We have $\sum_{h=j}^\infty [\alpha'_h - \delta'_h] = b + \sum_{h=j}^\infty [\alpha_h - \delta_h] \leq b + \sum_{h=j}^\infty \beta_h = \sum_{h=j}^\infty \beta_h'$.
\end{proof}

\ifreport
\begin{proof}[Proof of Lemma \ref{lemG4}]
\else
\begin{proof}[of Lemma \ref{lemG4}]
\fi
Consider any busy period $[\tau,\nu)$ of policy $P'$. Then, in policy $P'$, all servers are busy during $[\tau,\nu)$, and are idle at time $\tau^-$ and time $\nu$. We prove \eqref{eq_lemG4} for $t\in[\tau,\nu)$ by considering two cases:

\emph{Case 1: At time $t=\tau^-$, policy FUT-NR has $m$ tasks and the service of these tasks has just started.} Consider the system states of both policies at time $\tau^-$. The system state of policy FUT-NR satisfies 
\begin{align}\label{proof_lemG4_1}
\sum_{h=1}^\infty \alpha_h(\tau^-)= m, ~\bm{\alpha}(\tau^-)=\bm{\delta}(\tau^-).
\end{align}
In policy $P'$, there is no task in the system at time $\tau^-$ such that 
\begin{align}\label{proof_lemG4_5}
\bm{\beta}(\tau^-)=\bm{0}. 
\end{align}
Consider the evolutions of both policies during $[\tau,\nu)$. 
In policy $P'$, all servers are busy if there is at least one task. On the other hand, in policy FUT-NR, there is no task replication. Hence, all servers are busy if there are no less than $m$ tasks. Because the servers become busy in policy $P'$ at time $\tau$, a job must has arrived. By \eqref{proof_lemG4_1} and \eqref{proof_lemG4_5}, it holds that for $t=\tau$
%^there are no less than $m$ tasks in policy FUT-NR at time $\tau^-$.
\begin{align}\label{proof_lemG4_4}
\sum_{h=1}^\infty \alpha_h(t)= \sum_{h=1}^\infty \beta_h(t) +m\geq m+1.
\end{align}
Therefore,  the servers are all busy in policy $P'$ and policy FUT-NR at time $\tau$. Hence, for any sample path of policy $P'$, there is a sample path of policy FUT-NR such that for sufficiently small $\Delta t$ the task arrival times and task completion times of the two policies are exactly the same during $[\tau,\tau+\Delta t)$, and \eqref{proof_lemG4_4} holds during $[\tau,\tau+\Delta t)$. By induction over time, we can show that for any sample path of policy $P'$, there is a sample path of policy FUT-NR with the same probability density such that the task arrival times and task completion times of the two policies are exactly the same  during $[\tau,\nu)$, and \eqref{proof_lemG4_4} holds for all $t\in[\tau,\nu)$. Using Lemma \ref{lem_non_prmp1}, Lemma \ref{lem_non_prmp2}, and the initial states at time $\tau^-$, we can prove that \eqref{eq_lemG4} holds for all $t\in[\tau,\nu)$ on these two sample paths.

%In general, suppose that at some time $t\in[\tau,\nu)$
%\begin{align}
%\sum_{h=1}^\infty \alpha_h(t)= \sum_{h=1}^\infty \beta_h(t) +m\geq m+1.\nonumber
%\end{align}
%Then, the scheduling decisions of policies $P'$ and policy FUT-NR are the same at time $t$. This further implies that for any sample path of policy $P'$, we can construct a sample path of policy FUT-NR such that 
%\begin{align}
%\sum_{h=1}^\infty \alpha_h(t^+)= \sum_{h=1}^\infty \beta_h(t^+) +m\geq m+1.\nonumber
%\end{align}
%Therefore, 
%
%Using Lemma \ref{lem_non_prmp1} and Lemma \ref{lem_non_prmp2}, and we can prove that 
%\begin{align}
%\sum_{h=1}^\infty \alpha_h(t^+)= \sum_{h=1}^\infty \beta_h(t^+) +m.\nonumber
%\end{align}
%
%For any sample path of policy $P'$ during $[\tau,\nu)$, we can construct a sample path of policy FUT-NR during $[\tau,\nu)$ with the same probability density such that the task arrival times and task completion times of the two policies are exactly the same. In particular, if 
%
%
%if policy $P'$ has $b$ tasks at time $t\in[\tau,\nu)$, policy FUT-NR has $m+b$ tasks at time $t$. Hence, the scheduling decisions of policies $P'$ and policy FUT-NR are the same at time $t$. Therefore, we can obtain
%\begin{align}
%\sum_{h=1}^\infty \alpha_h(t)= \sum_{h=1}^\infty \beta_h(t) +m,~\forall~t\in [\tau,\nu).\nonumber
%\end{align}
%Because the task arrivals and departures of policies $P'$ and FUT-NR are aligned during $[\tau,\nu)$, using Lemma \ref{lem_non_prmp1}, Lemma \ref{lem_non_prmp2}, and the initial states at time $\tau^-$, we can prove by induction that \eqref{eq_lemG4} holds for $t\in[\tau,\nu)$.

\emph{Case 2: At time $t=\tau^-$, policy FUT-NR has less than $m$ tasks or the service of these tasks started before time $\tau^-$}. In both \emph{Case 1} and \emph{Case 2}, the sample path evolutions of policy $P'$ are the same. On the other hand, in policy FUT-NR, the tasks are completed earlier in \emph{Case 2} than in \emph{Case 1}. Therefore, \eqref{eq_lemG4} also holds in \emph{Case 2} for $t\in[\tau,\nu)$.

%Note that the case that policy FUT-NR has more than $m$ tasks at time $\tau^-$ will not happen. This will be clear 
Let $[\tau_1,\nu_1)$ be the next busy period of policy $P'$ with $\nu<\tau_1$. Then, $[\nu,\tau_1)$ is an idle period of policy $P'$. We prove \eqref{eq_lemG4} during the idle period $[\nu,\tau_1)$. 
Because all servers are idle during $[\nu,\tau_1)$ in policy $P'$, it follows that 
\begin{align}\label{proof_lemG4_2}
\bm{\beta}(t)=\bm{0},~t\in[\nu,\tau_1).
\end{align}
Hence, there is no task arrival during $[\nu,\tau_1)$; otherwise, \eqref{proof_lemG4_2} cannot be true.
On the other hand, at time $\nu$ there are no more than $m$ tasks in policy FUT-NR such that 
\begin{align}
\bm{\alpha}(\nu)=\bm{\delta}(\nu).\nonumber
\end{align}
Because there is no task arrival during $[\nu,\tau_1)$, policy FUT-NR satisfies
\begin{align}\label{proof_lemG4_3}
\bm{\alpha}(t)=\bm{\delta}(t),~t\in[\nu,\tau_1).
\end{align}
By \eqref{proof_lemG4_2} and \eqref{proof_lemG4_3}, \eqref{eq_lemG4} holds during $[\nu,\tau_1)$.
Further, from \eqref{proof_lemG4_3}, we can obtain
\begin{align}
\sum_{h=1}^\infty \alpha_h(\tau_1^-)=\sum_{h=1}^\infty \delta(\tau_1^-)\leq m,
\end{align}
such that there are no more than $m$ tasks at time $t=\tau_1^-$ in policy FUT-NR. Hence, either \emph{Case 1} or \emph{Case 2} is satisfied at time $t=\tau_1^-$. Then, we can use the above arguments to prove that  \eqref{eq_lemG4} holds during the next busy period $[\tau_1,\nu_1)$ of policy $P'$.

Finally, by taking an induction over the busy and idle periods of policy $P'$,  Lemma \ref{lemG4} is proven.
%Let $[\nu,\tau_1)$ and $[\tau_1,\nu_1)$ be the next idle and busy periods of policy $P'$, respectively. Because policy $P'$ is work-conserving, all $m$ servers are idle in policy $P'$ during $[\nu,\tau_1)$. Hence, there is no job arrival during $[\nu,\tau_1)$. At time $\nu$, we have
%\begin{align}
%\sum_{h=j}^\infty [\alpha_h(\nu)- \delta_h(\nu)]\leq 0.\nonumber
%\end{align}
%This and $\alpha_h(\nu)\geq\delta_h(\nu)$ imply that $\alpha_h(\nu)=\delta_h(\nu)$ for all $h=1,2,\ldots$ Since no job arrives during $[\nu,\tau_1)$, we can obtain that $\alpha_h(t)=\delta_h(t)$ for all $t\in[\nu,\tau_1)$ and $h=1,2,\ldots$ Hence, \eqref{eq_lemG4} holds during $[\nu,\tau_1)$. 
%
%Because there is no job arrival during $[\nu,\tau_1)$, there are no more than $m$ remaining tasks in FUT-NR at time $\tau_1$ and each remaining task has been processed by a certain amount of time. Similar with the case of $[\tau,\nu)$, we can prove that \eqref{eq_lemG4} holds in the busy period $[\tau_1,\nu_1)$.
%By taking an induction over the busy and idle periods of policy $P'$, Lemma \ref{lemG4} follows.
\end{proof}

\ifreport
\begin{proof}[Proof of Condition 3]
\else
\begin{proof}[of Condition 3]
\fi
%Let the evolution of the system state under some scheduling policy be on a space $(\Omega,\mathcal{F},P)$. Each $\omega\in\Omega$ corresponds to a sample path of policy $P'$ and a sample path of policy FUT-NR. The job arrival parameters $\mathcal{I}$ is fixed for all $\omega\in\Omega$. 
%Let $(C_{(1)}(P'),\ldots,c_{N:N}(P'))$ be a permute of the job completion time sequence $(c_{1}(P'),\ldots,c_{N}(P'))$ in the increasing order, such that $c_{i:N}(P')\leq c_{i+1:N}(P')$. 

%Pick any $\omega\in\Omega$ and consider the first job completion time $C_{(1)}(P')$ of policy $P'$. Suppose that there are $y$ job arrivals during $[0,C_{(1)}(P'))$. 

We will prove Condition 3 by induction. Consider the sample paths of policy $P'$ and policy FUT-NR satisfying Lemma \ref{lemG4}. We first show that there exists a job $w_1$ such that
\begin{align}\label{eq_Condition_3_1}
U_{w_1}(\text{FUT-NR}) \leq C_{(1)}(P').
\end{align}

In policy $P'$, the first job departure occurs at time $t=C_{(1)}(P')$. Suppose that $y_1$ jobs have arrived during $[0,C_{(1)}(P'))$. Then, there are $y_1-1$ unfinished jobs at time $C_{(1)}(P')$ in policy $P'$. Hence, the system state of policy $P'$ satisfies 
\begin{align}\label{eq_proof_0}
\sum_{h=y_1}^\infty\beta_h(C_{(1)}(P'))=0.
\end{align}
This and Lemma \ref{lemG4} imply
%Hence, there are $y-1$ unfinished jobs at time $C_{(1)}(P')$ such that
%Invoking Lemma \ref{lemG4}, we can obtain
\begin{align}\label{eq_proof_1}
\sum_{h=y_1}^\infty \alpha_h(C_{(1)}(P'))\leq \sum_{h=y_1}^\infty  \delta_h(C_{(1)}(P')).
\end{align}
In policy FUT-NR, there are at most $y_1$ jobs at time $C_{(1)}(P')$. Hence, the system state of policy FUT-NR must satisfy
\begin{align}\label{eq_proof_2}
\!\!\alpha_h(C_{(1)}(P'))= \delta_h(C_{(1)}(P'))=0,\forall~h=y_1\!+\!1,y_1\!+\!2,\ldots \!\!
\end{align}
Combining \eqref{eq_proof_1}, \eqref{eq_proof_2}, and the fact that $\alpha_h(t)\geq\delta_h(t)$ for all $h$ and $t$, we can obtain
%Combining \eqref{eq_proof_0}, \eqref{eq_proof_1}, and the fact that $\alpha_h(t)\geq\delta_h(t)$ for all $i,t$, yields
\begin{align}\label{eq_proof_3}
\alpha_{y_1}(C_{(1)}(P'))=\delta_{y_1}(C_{(1)}(P')).
\end{align}
Let $w_1$ be the index of the job associated to the $y_1$-th coordinate of $\bm{\alpha}(t)$ at time $t= C_{(1)}(P')$. Then, \eqref{eq_proof_3} tells us that in FUT-NR, all tasks of job $w_1$ are either completed or under service at time $C_{(1)}(P')$. Hence, \eqref{eq_Condition_3_1} is proven.
%\begin{align}%\label{eq_proof_9}
%U_{w_1}(\text{FUT-NR}) \leq C_{(1)}(P'),\nonumber
%\end{align}
%which implies \eqref{eq_Condition_3_1}.

Next, we prove the induction step. Suppose that there exist $j$ jobs indexed by $w_1,w_2,\ldots,w_j$ such that
\begin{align}
U_{w_i}(\text{FUT-NR}) \leq C_{(i)}(P'),~i=1,\ldots,j,\nonumber
\end{align}
we will show that there exist another job $w_{j+1}$ such that
\begin{align}\label{eq_proof_9}
U_{w_{j+1}}(\text{FUT-NR}) \leq C_{(j+1)}(P').
\end{align}
%Since preemption is not allowed, these $\delta_y(C_{(1)}(P'))$ tasks will be under service in policy FUT-NR until completion. Let $w_1$ be the index of the job associated to the coordinate $y$ at time $C_{(1)}(P')$. According to \eqref{eq_def_state}, we can obtain $\delta_y(C_{(1)}(P'))\leq \min[k_{w_1},M].$ Therefore, the time duration between $C_{(1)}(P')$ and $c_{w_1,\text{FUT-NR}}$ is no more than the time to complete $\min[k_{w_1},M]$ tasks of job $w_1$.
Assume that $y_{j+1}$ jobs have arrived during $[0,C_{(j+1)}(P'))$, which must satisfy $y_{j+1}\geq j+1$. Then, 
there are $(y_{j+1}-j-1)$ unfinished jobs at time $C_{(j+1)}(P')$ in policy $P'$. According to \emph{Definition \ref{def_state_P}}, the system state of policy $P'$ satisfies 
\begin{align}
\sum_{h=y_{j+1}-j}^\infty\beta_h(C_{(j+1)}(P'))=0.\nonumber
\end{align}
Then, by following the arguments of \eqref{eq_proof_1}-\eqref{eq_proof_3}, we can obtain that at time $t=C_{(j+1)}(P')$ the system state of policy FUT-NR satisfies
\begin{align}\label{eq_proof_4}
\alpha_{h}(C_{(j+1)}(P'))=\delta_{h}(C_{(j+1)}(P')),~h=y_{j+1}-j,\ldots,y_{j+1}.
\end{align}
There are $j+1$ jobs satisfying \eqref{eq_proof_4}. At least one of these $j+1$ jobs is different from the jobs $w_1,w_2,\ldots,w_j$. Let $w_{j+1}$ be the index of this job. Then, \eqref{eq_proof_4} tells us that in FUT-NR, all tasks of job $w_{j+1}$ are either completed or under service at time $t=C_{(j+1)}(P')$. Hence, \eqref{eq_proof_9} is proven.

By induction, we can obtain
\begin{align}\label{eq_proof_10}
U_{w_{j}}(\text{FUT-NR}) \leq C_{(j)}(P'),~j=1,\ldots,n.
\end{align}
Because $U_{(j)}(\pi)$ is the $j$-th smallest components of $\bm{U}(\pi)$, it follows that
\begin{align}\label{eq_proof_11}
U_{(j)}(\text{FUT-NR})\! \leq \!\max_{i=1,\ldots,j}U_{w_{j}}(\text{FUT-NR}),~j=1,\ldots,n.\!\!
\end{align}
Combining \eqref{eq_proof_10} and \eqref{eq_proof_11}, we obtain that for each sample path of policy $P'$, there is a sample path of policy FUT-NR with the same probability density such that 
\begin{align}
\bm{U}_{\uparrow}(\text{FUT-NR}) \leq  \bm{C}_{\uparrow}(P').
\end{align}
Considering all possible sample paths of these two policies, the stochastic ordering result in \eqref{eq_condition3} follows.
\end{proof}
After establishing conditions 1-3 of Lemma \ref{lem1} for policy FUT-NR,  we can use Lemma \ref{lem1} and Corollary \ref{coro1} to obtain \eqref{eq_delaygap1}. This completes the proof.

\subsection{Proof of {\large \eqref{eq_delaygap2}} in Theorem \ref{thm1}} 
The proof of \eqref{eq_delaygap2} is  similar with that of \eqref{eq_delaygap1} in Appendix \ref{sec_app_thm1_1}, except for the following two differences: 

First, policy FUT-NR in Appendix \ref{sec_app_thm1_1} should be replaced by policy FUT-NIR.

Second, task replications are allowed in policy FUT-NIR, which will introduce some extra delay to cancel the redundant task copies. %It is important to keep the cancellation overhead small. Otherwise, 
If the cancellation overhead is large, the servers might be busy cancelling the redundant task copies, instead of serving new tasks. In this case, Lemma \ref{lemG4} does not hold. Hence, we should keep the cancellation overhead small. In the design of policy FUT-NIR, a task replica is cancelled if the time to cancel the replica is stochastically shorter than the time to complete the replica; otherwise, the replica will not be cancelled. Using this and the extra conditions {$\bm{O}_{\mathcal{S}}\leq_{\text{st}}[\bm{X}_{\mathcal{S}}-\bm{\tau}_{\mathcal{S}}| \bm{X}>\bm{\tau}]$} and  {$\bm{O}_{\mathcal{S}^c}\geq_{\text{st}}[\bm{X}_{\mathcal{S}^c}-\bm{\tau}_{\mathcal{S}^c}| \bm{X}>\bm{\tau}]$}, we can obtain that in policy FUT-NIR the redundant task copies are completed stochastically earlier than processing these task copies until completion. Using this, the proof arguments of Lemma \ref{lemG4} also work for policy FUT-NIR.

\subsection{Proof of Corollary 3}  
Under the conditions of Corollary \ref{coro3}, policy FUT-NR satisfies the following three properties: (i) all $m$ servers are busy at all time $t\in[0,\infty)$, (ii) there is no task replications, and (iii) any completed task is from a job with the fewest remaining task. Therefore, policy FUT-NR is identical with policy $P'$ constructed in Appendix \ref{sec_app_thm1_1}. In addition, because there are at least $m$ remaining tasks at all time $t\in[0,\infty)$, policy FUT-NIR is identical with policy FUT-NR. Then, \eqref{eq_coro3} follows from Lemma \ref{lem1} and Corollary \ref{coro1}. 

%The details are provided in Appendix \ref{app2}.

%\textbf{Condition 4:} $P\in\Pi$. This condition is trivial. Hence, \eqref{eq_delaygap1} follows from Lemma \ref{thm2}.
%
%The remaining task is to prove \eqref{eq_delaygap2}. Since the $X_l$'s are independent NBU random variables with mean $\mathbb{E}[X_l]=1/\mu_l$, by Theorem 3.A.55 of \cite{StochasticOrderBook}, we can obtain
%\begin{align}
%X_l \leq_{\text{icx}} Z_l,~l=1,\ldots,m,\nonumber
%\end{align}
%where $\leq_{\text{icx}}$ is the increasing convex order defined in \cite[Chapter 4]{StochasticOrderBook} and the $Z_l$'s are independent exponential random variables with mean $\mu_l$. By Corollary 4.A.16 of \cite{StochasticOrderBook}, we have 
%\begin{align}
%\max_{l\in S} X_l \leq_{\text{icx}} \max_{l\in S} Z_l,~\forall~S\subseteq\{1,\ldots,m\}.\nonumber
%\end{align}
%Then, Eq. (4.A.1) of \cite{StochasticOrderBook} and $\mu_1\leq \ldots\leq \mu_M$ tell us that  
%\begin{align}
%\!\!\max_{\substack{S: |S|\leq k_i\\
%S\subseteq\{1,\ldots,m\}}}\!\!\mathbb{E}\!\left[\max_{l\in S} X_l\right]\!\leq\!\mathbb{E}\!\left[\max_{l=1,\ldots,k_i \wedge M} Z_l\right]\!\leq\!\sum_{l=1}^{k_i \wedge M} \frac{1}{\sum_{m=1}^l \mu_l}.\nonumber
%\end{align}
%This and \eqref{eq_proof_5} imply \eqref{eq_delaygap2}. This completes the proof.
