# Supplementary material for: Near Delay-Optimal Scheduling of Batch Jobs in Multi-Server Systems
Source: arXiv:2309.16880 source file (2023-09-28)
Supplement: Supplementary file 3 [file appendices_3.tex]

% !TEX root = ./replication.tex

\section{Proof of Thoerem~\ref{thm2}} \label{app2}
%\subsection{Proof of Thoerem~2} \label{sec_app_thm2_1}
%\subsection{Proof of Theorem \ref{thm2}}  
Define $\bm{s}=(s_{1},\ldots,$ $ s_{k_{\text{sum}}})$ as the sequence of task arrival times where $s_1\leq \ldots\leq s_{k_{\text{sum}}}$. Hence, $\bm{s}$ is determined by the job arrival times $a_1,\ldots,a_n$ and job sizes $k_1,\ldots,k_n$.
Recall that $\bm{T}_\pi=(T_{1,\pi},\ldots,$ $ T_{k_{\text{sum}},\pi})$ is the sequence of task completion times in policy $\pi$ where $T_{1,\pi}\leq \ldots\leq T_{k_{\text{sum}},\pi}$. 
We  first show that for all $\pi\in\Pi$
\begin{align}\label{eq_thm2_proof1}
[\bm{T}_{\text{FUT-R}}|\mathcal{I}] \leq_{\text{st}} [\bm{T}_\pi|\mathcal{I}].
\end{align}
We prove \eqref{eq_thm2_proof1} by induction. Consider the first task completion time $T_{1,\pi}$. Job 1 arrives at time $a_1=0$. All policy $\pi\in\Pi$ are non-preemptive. If policy $\pi$ is  work-conserving, then
\begin{align}
[T_{1,\pi}|\mathcal{I}]=\min_{l=1,\ldots,m} X_l,\nonumber
\end{align} 
otherwise, if policy $\pi$ is non-work-conserving, then
\begin{align}
[T_{1,\pi}|\mathcal{I}]\geq\min_{l=1,\ldots,m} X_l,\nonumber
\end{align} 
because of the possibility of server idleness. Since policy FUT-R$\in\Pi$ is work-conserving, we can obtain that for all $\pi\in\Pi$
\begin{align}\label{eq_thm2_condition1_2}
[T_{1,\text{FUT-R}}|\mathcal{I}]=\min_{l=1,\ldots,m} X_l\leq[T_{1,\pi}|\mathcal{I}].
\end{align} 

Next, consider the system evolution from $T_{j,\pi}$ to $T_{j+1,\pi}$. For any work-conserving policy $\pi\in\Pi$, we can obtain
\begin{eqnarray}\label{eq_thm2_2}
T_{j+1,\pi}\!=\max\{s_{j+1},T_{j,\pi}\} + \!\min_{l=1,\ldots,m} R_{j,l,\pi},
\end{eqnarray}
where $R_{j,l,\pi}$ is the time duration for server $l$ to complete a task since time $\max\{s_{j+1},T_{j,\pi}\}$. Suppose that server $l$ has spent $\tau_{l,\pi}$ ($\tau_{l,\pi}\geq0$) seconds on a task by time $\max\{s_{j+1},T_{j,\pi}\}$. 

Because the task service times are independent across the servers and the complementary CDF $\bar{F}$  is absolutely continuous, the probability for any two servers to complete their tasks at the same time is zero. Hence, $\Pr[R_{j,l,\pi} > 0] = 1$.\footnote{If $\bar{F}$  is not absolutely continuous, then it may happen that $\Pr[R_{j,l,\pi} > 0] < 1$ and two servers complete task executions at the same time. In this case, it is better to assign two distinct tasks than two replicated copies of the same task on these two servers.}
Therefore, in policy FUT-R, when a task copy is completed on a server, the remaining $m-1$ replicated copies of this task are still being processed on the other servers. Then, these replicated task copies are cancelled immediately and the servers are assigned to process $m$ replicated copies of a new task. 
Hence, $\tau_{l,\text{FUT-R}}=0$ for $l=1,\ldots,m$. The complementary CDF for the servers to complete a task after time $\max\{s_{j+1},T_{j,\text{FUT-R}})\}$ is 
\begin{align}\label{eq_thm2_7}
&\Pr\Big[\min_{l=1,\ldots,m} R_{j,l,\text{FUT-R}}>t\Big]\nonumber\\
=& \Pr\Big[\min_{l=1,\ldots,m}X_l>t \Big].
\end{align}
If $\pi$ is a work-conserving policy, then we have $\tau_l\geq0$ for $l=1,\ldots,m$. Hence, the tail probability for the servers to complete a task after time $\max\{s_{j+1},T_{j,\pi}\}$ is 
\begin{align}\label{eq_thm2_8}
&\Pr\Big[\min_{l=1,\ldots,m} R_{j,l,\pi}>t\Big]\nonumber\\
=& \Pr\Big[\min_{l=1,\ldots,m}(X_l-\tau_l)>t\Big|X_l> \tau_l, l=1,\ldots,m \Big].
\end{align} 
By \eqref{eq_thm2_7}, \eqref{eq_thm2_8}, and the task service times are independent NWU, yields 
\begin{align}\label{eq_min_thm2}
\min_{l=1,\ldots,m} R_{j,l,\text{FUT-R}}\leq_{\text{st}} \min_{l=1,\ldots,m} R_{j,l,\pi}.
\end{align}
Using \eqref{eq_thm2_2}, \eqref{eq_min_thm2}, and the fact that $s_j$ is uniquely determined by $\mathcal{I}$, it follows that for all work-conserving policy $\pi\in\Pi$
\begin{align}\label{eq_thm2_4}
[T_{j+1,\text{FUT-R}} | \mathcal{I},  T_{j,\text{FUT-R}}= t_j] \leq_{\text{st}} [T_{j+1,\pi} | \mathcal{I},  T_{j,\pi} = t_j'] \nonumber\\
\text{whenever}~ t_j \leq t_j',j=1,2,\ldots
\end{align}
If policy $\pi$ is non-work-conserving, \eqref{eq_thm2_2} becomes
\begin{eqnarray}\label{eq_thm2_2_1}
T_{j+1,\pi}\!\geq\max\{s_{j+1},T_{j,\pi}\} + \!\min_{l=1,\ldots,m} R_{j,l,\pi},\nonumber
\end{eqnarray}
because of the possibility of server idleness. In this case, \eqref{eq_thm2_4} still holds. Hence, \eqref{eq_thm2_4} holds for all $\pi\in\Pi_{\text{non-prmp}}$.
Then, combining \eqref{eq_thm2_condition1_2}, \eqref{eq_thm2_4}, and Theorem 6.B.3 of \cite{StochasticOrderBook}, yields
\begin{align}%\label{eq_thm1_5}
[(T_{1,\text{FUT-R}},\ldots,T_{j,\text{FUT-R}})|\mathcal{I}] \leq_{\text{st}} [(T_{1,\pi},\ldots,T_{j,\pi})|\mathcal{I}],~\forall~\pi\in\Pi.\nonumber
\end{align}
Hence, \eqref{eq_thm2_proof1} is proven.

According to Theorem 6.B.1 of \cite{StochasticOrderBook}, for any policy $\pi\in\Pi$, there exist that FUT-R$_1$ and policy $\pi_1$ which satisfy the same queueing disciplines and stochastic laws with policy FUT-R and policy $\pi$, and policy FUT-R$_1$ is more work-efficient than policy $\pi_1$ with probability one. Because each task is replicated on all $m$ servers and $k_1\leq \ldots\leq k_n$, each task completing service is from the job with the fewest remaining tasks among all unfinished jobs.
By Proposition \ref{lem1_0}, for all $f\in\mathcal{D}_{\text{sym}}$
\begin{align}
\Pr[f(\bm{C}(\text{FUT-R}_1)) \leq f(\bm{C}(\pi_1)) |\mathcal{I}]=1. \nonumber
\end{align}
Then, by Theorem 1.A.1 of \cite{StochasticOrderBook}, we can obtain \eqref{eq_delaygap3}, which completes the proof.

\section{Proof of Lemma \ref{lem7_NWU}}\label{app_lem7_NWU}  
Consider the time difference ${C}_i(\text{FUT-R})-{U}_i(\text{FUT-R})$.
%\textbf{Condition 4:} $P\in\Pi$. This condition is trivial. Hence, \eqref{eq_delaygap1} follows from Lemma \ref{thm2}.
In policy FUT-R, all servers are allocated to process $m$ replicated copies of a task from the job with the fewest unassigned tasks. Hence, at time ${U}_i(\text{FUT-R})$, one task of job $i$ are being processed by all $m$ servers. 
%Then, $\mathcal{S}_i$ is a random set with cardinality $|\mathcal{S}_i|\leq k_i\wedge m$.
%The remaining task is to prove \eqref{eq_delaygap2}. 
Because the $X_l$'s are independent exponential random variables with mean $\mathbb{E}[X_l]=1/\mu_l$, 
by Theorem 3.A.55 of \cite{StochasticOrderBook}, we can obtain
%\begin{align}
%X_l \leq_{\text{icv}} Z_l,~l=1,\ldots,m,\nonumber
%\end{align}
%where $\leq_{\text{icv}}$ is the increasing concave order defined in \cite[Chapter 4]{StochasticOrderBook} and the $Z_l$'s are independent exponential random variables with mean $\mathbb{E}[Z_l]=\mu_l$. By Corollary 4.A.16 of \cite{StochasticOrderBook}, we have 
%\begin{align}\label{eq_exp_orderNWU}
%\min_{l=1,\ldots,m} X_l \leq_{\text{icv}} \min_{l=1,\ldots,m} Z_l.
%\end{align}
%Note that the set $\mathcal{S}_i$ is determined by the evolution of policy FUT-R up to time ${U}_i(\text{FUT-R})$.Because the task service times are determined by an external process which is not affected by the scheduling policy FUT-R, $X_l$ and $Z_l$ are independent of $\mathcal{S}_i$ for each $l\in \mathcal{S}_i$.
%Then,   
\begin{align}
&\mathbb{E}[{C}_i(\text{FUT-R})-{U}_i(\text{FUT-R})|\mathcal{I}]\nonumber\\
\leq &\mathbb{E}\!\left[\min_{l=1,\ldots,m} X_l\bigg|\mathcal{I}\right]\label{eq_gap_NWU_condition1}\\
=&\mathbb{E}\!\left[ \min_{l=1,\ldots,m} X_l\right]\label{eq_gap_NWU_condition2}\\
%\leq&\mathbb{E}\!\left[ \min_{l=1,\ldots,m} Z_l\right]\label{eq_gap_NWU_condition3}\\
\leq &\frac{1}{\sum_{l=1}^m \mu_l}.\label{eq_gap_NWU_condition5}
\end{align}
where \eqref{eq_gap_NWU_condition1} is because one task of job $i$ are being processed by all $m$ servers at time ${U}_i(\text{FUT-R})$, \eqref{eq_gap_NWU_condition2} is because $X_l$ is independent of $\mathcal{I}$, 
%\eqref{eq_gap_NWU_condition3} is due to\eqref{eq_exp_orderNWU} and Eq. (4.A.1) of \cite{StochasticOrderBook}, 
and \eqref{eq_gap_NWU_condition5} is due to the property of exponential distributions. By this, Lemma \ref{lem7_NWU} is proven.
