# Supplementary material for: Near Delay-Optimal Scheduling of Batch Jobs in Multi-Server Systems
Source: arXiv:2309.16880 source file (2023-09-28)
Supplement: Supplementary file 4 [file appendices_3version2.tex]

% !TEX root = ./replication.tex

\section{Proofs of Proposition~\ref{coro3_1}} \label{app0_2}
%\ifreport
%\begin{proof}[Proof of Thoerem \ref{lem3}]
%\else
%\begin{proof}[of Thoerem \ref{lem3}]
%\fi
%Thoerem \ref{lem3} follows from Thoerem \ref{lem2} by letting $d_i=a_i$ for all $i$.
%\end{proof}
%\ifreport
%\begin{proof}[Proof of Corollary~\ref{coro3_1}]
%\else
%\begin{proof}[of Corollary~\ref{coro3_1}]
%\fi
%Proposition~\ref{coro3_1} follows from Corollary \ref{coro2} by letting $d_i=a_i$ for all $i$.
%As in the proof of Corollary \ref{coro2}, let $w_i$ denote the index of the job associated with $v_{(i)}(P)$.
%
%We assume that the arrival times $a_1,\ldots, a_n$ of the $n$ jobs are distinct from each other. This does not lose any generality, because if $a_i=a_j$ for two jobs $i$ and $j$, Proposition~\ref{coro3_1} can be proven by first proving for the case $a_i=a_j+\epsilon$ and then taking the limit $\epsilon\rightarrow 0$. 
We take 3 steps to prove Proposition~\ref{coro3_1}:

\emph{Step 1: We show that}  
%Thoerem \ref{lem3} holds if \emph{$D_{\max}(\cdot)$} is replaced by any $f\in\mathcal{D}_{\text{sym}}$.}
\begin{align}\label{eq_coro2_2_2}
v_{(i)}(P) \leq c_{(i)}(\pi),~i=1,\ldots,n.
\end{align}

In policy $P$, each unassigned task entering the servers is from the job with the earliest arrival time among all jobs with unassigned tasks. Because each job has $k$ tasks, in policy $P$ only the job with the earliest arrival time may have fewer than $k$ unassigned tasks, the other jobs arrived later have exactly $k$ unassigned tasks. Therefore, among all jobs with unassigned tasks, the job with the earliest arrival time is also the job with the fewest unassigned tasks.
Then, \eqref{eq_coro2_2_2} follows from Proposition~\ref{lem1}. 
In addition, we can use Proposition \ref{lem1} to prove that \eqref{eq_coro3_1_1} holds for all $f\in\mathcal{D}_{\text{sym}}$.

The remaining proof is almost identical with \emph{Step 2} and \emph{Step 3} in the proof of Proposition \ref{coro2}, except that $d_i$ should be replaced by $a_i$. 
By this, Proposition~\ref{coro3_1} is proven.
