# Supplementary material for: Near Delay-Optimal Scheduling of Batch Jobs in Multi-Server Systems
Source: arXiv:2309.16880 source file (2023-09-28)
Supplement: Supplementary file 7 [file appendices_lem1_0.tex]

\section{Proof of Proposition \ref{lem1_0}} \label{app_lem1_0}

The following two lemmas are needed to prove Proposition \ref{lem1_0}:  

\begin{lemma}\cite[Lemmas 1-2]{Smith78}\label{lem_non_prmp1_0}
Suppose that under policy $P$, $\{\bm{\xi}_{P}',\bm{\gamma}_{P}'\}$ is obtained by completing $b_P$ tasks in the system whose state is $\{\bm{\xi}_{P},\bm{\gamma}_{P}\}$. Further, suppose that under policy $\pi$, $\{\bm{\xi}_{\pi}',\bm{\gamma}_{\pi}'\}$ is obtained by completing $b_\pi$ tasks in the system whose state is $\{\bm{\xi}_{\pi},\bm{\gamma}_{\pi}\}$.
If $b_P\geq b_\pi$, policy $P$ satisfies condition 3 of Proposition \ref{lem1_0}, and 
\begin{eqnarray}\label{eq_non_prmp_41_0}
\sum_{i=j}^n {\xi}_{[i],P}\leq \sum_{i=j}^n {\xi}_{[i],\pi}, ~j = 1,2,\ldots,n,\nonumber
\end{eqnarray}
then
\begin{eqnarray}\label{eq_non_prmp_40_0}
\sum_{i=j}^n {\xi}_{[i],P}'\leq \sum_{i=j}^n {\xi}_{[i],\pi}', ~j = 1,2,\ldots,n.
\end{eqnarray}
\end{lemma}

\begin{lemma}\cite[Lemma 3]{Smith78}\label{lem_non_prmp2_0}
Suppose that, under policy $P$, $\{\bm{\xi}_{P}',\bm{\gamma}_{P}'\}$ is obtained by adding a job with $b$ tasks to the system whose state is $\{\bm{\xi}_{P},\bm{\gamma}_{P}\}$. Further, suppose that, under policy $\pi$, $\{\bm{\xi}_{\pi}',\bm{\gamma}_{\pi}'\}$ is obtained by adding a job with $b$ tasks to the system whose state is $\{\bm{\xi}_{\pi},\bm{\gamma}_{\pi}\}$.
If
\begin{eqnarray}
\sum_{i=j}^n {\xi}_{[i],P}\leq \sum_{i=j}^n {\xi}_{[i],\pi}, ~j = 1,2,\ldots,n,\nonumber
\end{eqnarray}
then
\begin{eqnarray}
\sum_{i=j}^n {\xi}_{[i],P}'\leq \sum_{i=j}^n {\xi}_{[i],\pi}', ~j = 1,2,\ldots,n.\nonumber
\end{eqnarray}
\end{lemma}

We now use Lemma \ref{lem_non_prmp1_0} and Lemma \ref{lem_non_prmp2_0} to prove Proposition \ref{lem1_0}.
\ifreport
\begin{proof}[Proof of Proposition \ref{lem1_0}]
\else
\begin{proof}[of Proposition \ref{lem1_0}]
\fi

Because policy $P$ is more work-efficient than policy $\pi$, the sequence of task completion times in policy $P$ are  smaller  than those in policy $\pi$, i.e., 
\begin{align}
(t_{1,P},\ldots, t_{k_{\text{sum}},P}) \leq(t_{1,\pi},\ldots, t_{k_{\text{sum}},\pi}). \nonumber
\end{align} 

We modify the sample-path of policy $P$ as follows:  Suppose that for each $i=1,\ldots, k_{\text{sum}}$  a task of job $j_i$ is completed at time $t_{i,P}$ on the original sample-path of policy $P$, then on the modified sample-path of policy $P$ a task of job $j_i$ is completed at time $t_{i,\pi}$. By this modification, the task completion times of policy $P$ are postponed, but the order of completed tasks remain the same. 
Let $\hat{\bm{\xi}}_{P}(t) =(\hat{\xi}_{1,P}(t),\ldots,\hat{\xi}_{n,P}(t))$ and $\hat{\bm{\gamma}}_{P}(t) =(\hat{\gamma}_{1,P}(t),\ldots,\hat{\gamma}_{n,P}(t))$ denote the system state on the modified sample-path of policy $P$. Because the task completion times are postponed,  we can get ${\xi}_{i,P}(t)  \leq \hat{\xi}_{i,P}(t) $ for all $t\geq 0$ and $i=1,\ldots,n$. Hence, for all $t\in[0,\infty)$
\begin{align}\label{eq_lem1_0_proof_1}
\sum_{i=j}^n {\xi}_{[i],P}(t)\leq \sum_{i=j}^n \hat{\xi}_{[i],P}(t), ~i=1,2,\ldots,n.
\end{align}

Next, we compare policy $\pi$ with the modified sample-path of policy $P$. By the foregoing modification, \emph{the task completion times are identical on the sample-path of policy $\pi$ and on the modified sample-path of policy $P$.} 
 
On the original sample-path of policy $P$, each task completing service  is from the job with the fewest remaining tasks among all jobs in the queue. On the modified sample-path of policy $P$, there are more jobs in the queue at the postponed   task completion times due to additional job arrivals. Because $k_1\leq k_2\leq \ldots\leq k_n$, later arrived jobs have more tasks. Hence, on the modified sample-path of policy $P$, each task completing service  is still from the job with the fewest remaining tasks among all jobs in the queue. In other words, \emph{condition 3 of Proposition \ref{lem1_0} is satisfied on the modified sample-path of policy $P$}. 

Because $\hat{\bm{\xi}}_{P}(0) = {\bm{\xi}}_{\pi}(0) =\bm{0}$, by using Lemma \ref{lem_non_prmp1_0} and Lemma \ref{lem_non_prmp2_0}, and taking an induction on the job arrival events and task completion events over time, we can obtain for all $t\in[0,\infty)$
% Then, by using the arguments in \cite{Smith78} we can show 
\begin{align}\label{eq_lem1_0_proof_2}
\sum_{i=j}^n \hat{\xi}_{[i],P}(t)\leq \sum_{i=j}^n {\xi}_{[i],\pi}(t), ~i=1,2,\ldots,n.
\end{align}
Combining \eqref{eq_lem1_0_proof_1} and \eqref{eq_lem1_0_proof_2}, yields \eqref{eq_ordering_1_1}. Then, \eqref{eq_ordering_1_1_2} and \eqref{eq_ordering_1_2} follow from Lemma \ref{ordering_1}, which completes the proof. \end{proof}
