# Supplementary material for: Near Delay-Optimal Scheduling of Batch Jobs in Multi-Server Systems
Source: arXiv:2309.16880 source file (2023-09-28)
Supplement: Supplementary file 8 [file appendices_lem2_0.tex]

\section{Proof  of Proposition \ref{lem2_0}} \label{app_lem2_0}

The proof of Proposition \ref{lem2_0} requires the following two lemmas:

\begin{lemma}\label{lem_non_prmp1_thm3_0}
Suppose that, in policy $P$, $\{\bm{\xi}_P',\bm{\gamma}_P'\}$ is obtained by completing $b_P$ tasks in the system whose state is $\{\bm{\xi}_P,\bm{\gamma}_P\}$. Further, suppose that, in policy $\pi$, $\{\bm{\xi}_\pi',\bm{\gamma}_\pi'\}$ is obtained by completing $b_\pi$ tasks in the system whose state is $\{\bm{\xi}_\pi,\bm{\gamma}_\pi\}$.
If $b_P\geq b_\pi$, condition 3 of Proposition \ref{lem2_0} is satisfied in policy $P$, and
\begin{eqnarray}
\sum_{i:d_i\leq\tau} \xi_{i,P}\leq \sum_{i:d_i\leq\tau} \xi_{i,\pi}, ~\tau\in[0,\infty),\nonumber
\end{eqnarray}
then
\begin{eqnarray}\label{eq_non_prmp_40_thm3_0}
\sum_{i:d_i\leq\tau} \xi_{i,P}'\leq \sum_{i:d_i\leq\tau} \xi_{i,\pi}', ~\tau\in[0,\infty).\end{eqnarray}
\end{lemma}

\begin{proof}
If $\sum_{i:d_i\leq\tau} \xi_{i,P}'=0$, then the inequality \eqref{eq_non_prmp_40_thm3} follows naturally. 
If $\sum_{i:d_i\leq\tau} \xi_{i,P}'>0$, then there exist some remaining tasks. 
In policy $P$, each task completing service is from the job with the earliest due time. Hence,
$\sum_{i:d_i\leq\tau} \xi_{i,P}'=\sum_{i:d_i\leq\tau} \xi_{i,P} - b_P \leq \sum_{i:d_i\leq\tau} \xi_{i,\pi} -b_\pi \leq \sum_{i:d_i\leq\tau} \xi_{i,\pi}'$.
\end{proof}

\begin{lemma}\label{lem_non_prmp2_thm3_0}
Suppose that under policy $P$, $\{\bm{\xi}_P',\bm{\gamma}_P'\}$ is obtained by adding a job with $b$ tasks and due time $d$ to the system whose state is $\{\bm{\xi}_P,\bm{\gamma}_P\}$. Further, suppose that under policy $\pi$, $\{\bm{\xi}_\pi',\bm{\gamma}_\pi'\}$ is obtained by adding a job with $b$ tasks and due time $d$ to the system whose state is $\{\bm{\xi}_\pi,\bm{\gamma}_\pi\}$.
If
\begin{eqnarray}
\sum_{i:d_i\leq\tau} \xi_{i,P}\leq \sum_{i:d_i\leq\tau} \xi_{i,\pi}, ~\tau\in[0,\infty),\nonumber
\end{eqnarray}
then
\begin{eqnarray}
\sum_{i:d_i\leq\tau} \xi_{i,P}'\leq \sum_{i:d_i\leq\tau} \xi_{i,\pi}', ~\tau\in[0,\infty).\nonumber\end{eqnarray}
\end{lemma}

\begin{proof}
If $d\leq\tau$, then
$\sum_{i:d_i\leq\tau} \xi_{i,P}'\leq \sum_{i:d_i\leq\tau} \xi_{i,P} + b\leq \sum_{i:d_i\leq\tau} \xi_{i,\pi}+b \leq \sum_{i:d_i\leq\tau} \xi_{i,\pi}'$.

If $d>\tau$, then
$\sum_{i:d_i\leq\tau} \xi_{i,P}'\leq \sum_{i:d_i\leq\tau} \xi_{i,P} \leq \sum_{i:d_i\leq\tau} \xi_{i,\pi} \leq \sum_{i:d_i\leq\tau} \xi_{i,\pi}'$.
\end{proof}

\begin{proof}[Proof of Proposition \ref{lem2_0}]

Because policy $P$ is more work-efficient than policy $\pi$, the task completion times in policy $P$ are smaller  than those in policy $\pi$, i.e., 
\begin{align}
(t_{1,P},\ldots, t_{k_{\text{sum}},P}) \leq(t_{1,\pi},\ldots, t_{k_{\text{sum}},\pi}). \nonumber
\end{align} 

We modify the sample-path of policy $P$ as follows:  Suppose that for each $i=1,\ldots, k_{\text{sum}}$  a task of job $j_i$ is completed at time $t_{i,P}$ on the original sample-path of policy $P$, then on the modified sample-path of policy $P$ a task of job $j_i$ is completed at time $t_{i,\pi}$. Hence, the task completion times of policy $P$ are postponed after the modification, but the order of completed tasks remain the same. 
Let $\hat{\bm{\xi}}_{P}(t) =(\hat{\xi}_{1,P}(t),\ldots,\hat{\xi}_{n,P}(t))$ and $\hat{\bm{\gamma}}_{P}(t) =(\hat{\gamma}_{1,P}(t),\ldots,\hat{\gamma}_{n,P}(t))$ denote the system state on the modified sample-path of policy $P$. Then, at any time $t$ we can get ${\xi}_{i,P}(t)  \leq \hat{\xi}_{i,P}(t) $ for $i=1,\ldots,n$ and hence
\begin{align}\label{eq_lem2_0_proof_1}
\sum_{i:d_i\leq\tau} {\xi}_{i,P}(t)\leq \sum_{i:d_i\leq\tau} \hat{\xi}_{i,P}(t), ~\tau\in[0,\infty).
\end{align}

Next, we compare policy $\pi$ with the modified sample-path of policy $P$. By the foregoing construction, \emph{the task completion times are identical on the sample-path of policy $\pi$ and on the modified sample-path of policy $P$.}
 
On the original sample-path of policy $P$, each task completing service  is from the job with the earliest due time among all jobs in the queue. Furthermore, because $k_1\leq k_2\leq \ldots\leq k_n$, later arrived jobs have more tasks. Hence, on the modified sample-path of policy $P$, each task completing service  is also from the job with the earliest due time among all jobs in the queue. In other words, \emph{condition 3 of Proposition \ref{lem2_0} is satisfied on the modified sample-path of policy $P$}. 

Because $\hat{\bm{\xi}}_{P}(0) = {\bm{\xi}}_{\pi}(0) =\bm{0}$, by using Lemma \ref{lem_non_prmp1_thm3_0} and Lemma \ref{lem_non_prmp2_thm3_0}, and taking an induction on the job arrival events and task completion events over time, we can obtain for all $t\in[0,\infty)$
% Then, by using the arguments in \cite{Smith78} we can show 
\begin{align}\label{eq_lem2_0_proof_2}
\sum_{i:d_i\leq\tau} \hat{\xi}_{i,P}(t)\leq \sum_{i:d_i\leq\tau} {\xi}_{i,\pi}(t), ~i=1,2,\ldots,n.
\end{align}
Combining \eqref{eq_lem2_0_proof_1} and \eqref{eq_lem2_0_proof_2}, yields \eqref{eq_ordering_3_1}. Then, \eqref{eq_ordering_3_2} follow from Lemma \ref{ordering_3}, which completes the proof. \end{proof}
