# Supplementary material for: Near Delay-Optimal Scheduling of Batch Jobs in Multi-Server Systems
Source: arXiv:2309.16880 source file (2023-09-28)
Supplement: Supplementary file 9 [file appendix_MNBU_property.tex]

% !TEX root = ./replication.tex

\section{Proof of Lemma 4}\label{app_MNBUproperty}
\begin{itemize}
\itemsep0em
\item[1-2.] Properties 1-2 directly follow from \emph{Definition \ref{MNBU}}. 

\item[3.] To show a given subset of random variables is MNBU (MNWU), set $\tau_i=-\infty$ for all random variables in the complementary set. By this, property 3 is proven.  

\item[4.] Property 4 can be proven by using \emph{Definition \ref{MNBU}}.

\item[5.] According to \eqref{eq_MNBU} and \eqref{eq_MNWU}, we can obtain 
\begin{align}\label{app_MNBUproperty_1}
\bar{F}(\bm{\tau}+t \bm{e})\leq \bar{F}(\bm{\tau})\bar{F}(t\bm{e})
\end{align}
for MNBU distributions and 
\begin{align}\label{app_MNBUproperty_2}
\bar{F}(\bm{\tau}+t \bm{e})\geq \bar{F}(\bm{\tau})\bar{F}(t\bm{e})
\end{align} for MNWU distributions, where $\bm{e}=(1,\ldots,1)$. In \cite{Ghurye1984}, it was shown that the only distribution satisfying both \eqref{app_MNBUproperty_1} and \eqref{app_MNBUproperty_2} must be the multivariate exponential distribution of Marshall and Olkin. Hence, property 5 is proven. 

\item[6.] According to \cite{Marshall1967}, the survival function of a multivariate exponential distribution of Marshall and Olkin is absolutely continuous if and only if its components are independent exponentials. By this, property 6 is proven.

\item[7.] If $\bm{X}$ is MNBU, then
\begin{align}\label{eq_property_MNBUMNWU1}
&\Pr\Big[\min_{l=1,\ldots,m}(X_l-\tau_l)>t\Big| \bm{X}> \bm{\tau} \Big]\nonumber\\
=& \Pr[\bm{X}>\bm{\tau}+t\bm{e}| \bm{X}> \bm{\tau} ]\nonumber\\
=& \frac{\Pr[\bm{X}>\bm{\tau}+t\bm{e}]}{\Pr[\bm{X}>\bm{\tau}]}\nonumber\\
\leq& \frac{\Pr[\bm{X}_{\mathcal{S}}>\bm{\tau}_{\mathcal{S}}+t\bm{e}_{\mathcal{S}}, \bm{X}_{\mathcal{S}^c}>t\bm{e}_{\mathcal{S}^c}]}{\Pr[\bm{X}_{\mathcal{S}}>\bm{\tau}_{\mathcal{S}}]}\\
=&\Pr\Big\{\min_{l\in\mathcal{S}}(X_l-\tau_l)>t,\min_{i\in\mathcal{S}^c}X_l>t \Big| \bm{X}_{\mathcal{S}}> \bm{\tau}_{\mathcal{S}}\Big\},\nonumber\\
=&\Pr\Big\{\min\Big[\min_{l\in\mathcal{S}}(X_l-\tau_l),\min_{i\in\mathcal{S}^c}X_l\Big]>t \Big| \bm{X}_{\mathcal{S}}> \bm{\tau}_{\mathcal{S}}\Big\},\nonumber
\end{align}
where $\bm{e}$ is an $m$-dimensional vector with all $1$ components, $\bm{e}_{\mathcal{A}}$  is a $|\mathcal{A}|$-dimensional vector with all $1$ components, and the inequality \eqref{eq_property_MNBUMNWU1} is obtained by using \eqref{eq_MNBU} iteratively for each $i\in\mathcal{S}^c$. Similar results can be obtained for MNWU distributions. By this, property 7 is proven.
\end{itemize}
%\end{proof}

%Define $\bm{s}=(s_{1},\ldots, s_{k_{\text{sum}}})$ as the sequence of task arrival times of the system, and $\bm{T}(\pi)=(T_{1}(\pi),\ldots,$ $ T_{k_{\text{sum}}}(\pi))$ as the sequence of task completion times of the system. The components of $\bm{s}$ and $\bm{T}(\pi)$ are arranged in the increasing order such that $\bm{s} =\bm{s}_{\uparrow}$ and $\bm{T}(\pi)=\bm{T}_{\uparrow}(\pi)$. Hence, $\bm{s}$ is uniquely determined by $\mathcal{I}$, while $\bm{T}(\pi)$ is determined by $\mathcal{I}$, the scheduling policy $\pi$, and random task service times.
%Then, $\bm{t}(\pi_1)\leq\bm{t}(\pi_2)$ holds on sample path if, and only if, $[\bm{T}(\pi_1)|\mathcal{I}] \leq_{\text{st}}[\bm{T}(\pi_2)|\mathcal{I}]$ for all $\mathcal{I}$.
