# Supplementary material for: Near Delay-Optimal Scheduling of Batch Jobs in Multi-Server Systems
Source: arXiv:2309.16880 source file (2023-09-28)
Supplement: Supplementary file 15 [file appendices_4.tex]

% !TEX root = ./replication.tex
%\section{Proofs of Thoerem~6 and Corollary 6} \label{app3}
%Similar with the proof of Theorem \ref{thm1}, we can show that policy EDD-NR and policy EDD-NIR are more work-efficient than any policy $\pi\in\Pi$. Then, Theorem \ref{thm3} follows from Thoerem \ref{lem2}, and Corollary \ref{coro_thm3_1} follows from Corollary \ref{coro2}.

%\section{Proofs of Thoerem~7 and Corollary 7} \label{app4}
%Similar with the proof of Theorem \ref{thm2}, we can show that policy EDD-R is more work-efficient than any policy $\pi\in\Pi$. Then, Theorem \ref{thm4} follows from Thoerem \ref{lem2}, and Corollary \ref{coro4_1} follows from Corollary \ref{coro2}.
%
%\section{Proofs of Thoerem~8 and Corollary 8} \label{app5}
%Similar with the proof of Theorem \ref{thm1}, we can show that policy FCFS-NR and policy FCFS-NIR are more work-efficient than any policy $\pi\in\Pi$. Then, Theorem \ref{thm5} follows from Thoerem \ref{lem3}, and Corollary \ref{coro5_1} follows from Corollary \ref{coro3_1}.
%
%\section{Proofs of Thoerem~9 and Corollary 9} \label{app6}
%Similar with the proof of Theorem \ref{thm2}, we can show that policy FCFS-R is more work-efficient than any policy $\pi\in\Pi$. Then, Theorem \ref{thm6} follows from Thoerem \ref{lem3}, and Corollary \ref{coro6_1} follows from Corollary \ref{coro3_1}.

%\end{proof}

%\subsection{Proof of Thoerem~\ref{thm3}} \label{sec_app_3_1} 
%We prove Thoerem~\ref{thm3} by using the sufficient conditions in Thoerem \ref{lem2}. The details are as follows:
%
%{\bf Construction of Policy $P'$:}
%We construct an {infeasible} policy $P'$. \emph{First, in policy $P'$, all servers are busy whenever the queue is not empty.} If the number of tasks is less than $m$, some tasks are replicated over multiple servers. 
%\emph{Second, the task completion times of policy $P'$ are constructed as if there is no task cancellations.} Suppose that at any time $t$, server $l$ has processed a task for $\tau$ seconds, and another copy of this task is completed at time $t$ on another server. In policy $P'$, server $l$ will cancel this task and process a new task. More specifically, in policy $P'$, server $l$ will not process the new task from scratch; instead, it is assumed that the new task assigned to server $l$ has already been processed for $\tau$ seconds by time $t$ (which is infeasible),~and server $l$ will serve the task from this progress point. If two task copies are completed  at the same time on two servers, these two task copies are assumed to be distinct tasks; that is, they are not replicated copy of each other.  \emph{Finally, the completed tasks of policy $P'$ are relabelled such that each completed task is from the job with the earliest due time}. (This relabeling operation might be infeasible, because the tasks from different jobs may be simultaneously processed on parallel servers.) By this, policy $P'$ is constructed.
%
%
%Next, we prove the conditions of Thoerem \ref{lem2} one by one.
%
%\textbf{Condition 1:} \emph{Policy $P'$ is more {work-efficient} than any policy $\pi\in\Pi$}. Condition 1 can be proven by using the same proof arguments in Appendix \ref{sec_app_thm1_1}.
%
%\textbf{Condition 2:} \emph{Each completed task of policy $P'$ belongs to the job with the earliest due time}. Condition 2 directly follows from the construction of policy $P'$.
%
%\textbf{Condition 3:} \emph{It holds that} 
%\begin{align}\label{eq_condition3_thm3}
%[\bm{U}_{}(\text{EDD-NR})|\mathcal{I}] \leq_{\text{st}} [\bm{C}_{}(P')|\mathcal{I}].
%\end{align}
%
%We prove condition 3 by using the \emph{sample-path ordering} technique. First, we define the system states of policies $P'$ and EDD-NR. 
%\begin{definition}\label{def_state_P_thm3}
%The system state of policy $P'$ is specified by a $n$-dimensional vector $\bm{\xi}=(\xi_1,\ldots,\xi_n)$ with non-negative components. At any time, if job $i$ exists in the system, $\xi_i$ is the number of remaining tasks of job $i$; if job $i$ has not arrived at the system or has departed from the system, $\xi_i=0$.
%\end{definition}
%
%\begin{definition}\label{def_state_thm3}
%The system state of policy EDD-NR is specified by a pair of $n$-dimensional vectors $\bm{\gamma}=(\gamma_1,\ldots,\gamma_n)$ and $\bm{\zeta}=(\zeta_1,\ldots,\zeta_n)$ with non-negative components. 
%At any time, if job $i$ exists in the system, then $\gamma_i$ is the number of remaining tasks of job $i$ and $\zeta_i$ out of these $\gamma_i$ tasks are under service on some servers; if job $i$ has not arrived at the system or has departed from the system, then $\gamma_i=\zeta_i=0$.
%Hence, 
%\begin{align}%\label{eq_def_state_thm3}
%\zeta_i  \leq \gamma_i \leq k_{i},~\sum_{i=1}^n \zeta_i \leq m. \nonumber
%\end{align}
%\end{definition}
%
% Let $\{\bm{\xi}(t),t\geq0\}$ be the state process of policy $P'$, and $\{\bm{\gamma}(t),\bm{\zeta}(t),t\geq0\}$ be the state process of EDD-NR, which are assumed to be right-continuous. During the proof of condition 3, we assume that the due times $d_1,\ldots, d_n$ of the $n$ jobs are distinct from each other. This does not lose any generality, because if $d_i=d_j$ for two jobs $i$ and $j$, condition 3 can be proven by taking the limit $d_i\rightarrow d_j$. 
%
%The sample-path ordering result is stated in the following lemma:
% 
% 
%\begin{lemma}\label{lemG4_thm3}
%Suppose that $\bm{\xi}(0^-)=\bm{\gamma}(0^-)=\bm{\zeta}(0^-)=\bm{0}$ and the job parameters $\mathcal{I}$ are given. For any sample path of policy $P'$, there exists a sample path of EDD-NR with the same probability density such that
%\begin{eqnarray}\label{eq_lemG4_thm3}
%\sum_{i:d_i\leq\tau} [\gamma_i(t) - \zeta_i(t)]\leq \sum_{i:d_i\leq\tau} \xi_i(t), 
%\end{eqnarray}
%holds for all $t,\tau\geq0$.
%\end{lemma}
%
%The following two lemmas are needed to prove Lemma \ref{lemG4_thm3}:
%
%
%\begin{lemma}\label{lem_non_prmp1_thm3}
%Suppose that, under policy EDD-NR, $\{\bm{\gamma}',\bm{\zeta}'\}$ is obtained by completing a task on one server in the system whose state is $\{\bm{\gamma},\bm{\zeta}\}$. Further, suppose that, under policy $P'$, $\bm{\xi}'$ is obtained by completing a task on one server in the system whose state is $\bm{\xi}$. If
%\begin{eqnarray}
%\sum_{i:d_i\leq\tau} [\gamma_i - \zeta_i]\leq \sum_{i:d_i\leq\tau} \xi_i, ~\forall~\tau\in[0,\infty),\nonumber
%\end{eqnarray}
%then
%\begin{eqnarray}\label{eq_non_prmp_40_thm3}
%\sum_{i:d_i\leq\tau} [\gamma_i'- \zeta_i']\leq \sum_{i:d_i\leq\tau} \xi_i', ~\forall~\tau\in[0,\infty).\end{eqnarray}
%\end{lemma}
%
%\begin{proof}
%If $\sum_{i:d_i\leq\tau} [\gamma_i' - \zeta_i']=0$, then the inequality \eqref{eq_non_prmp_40_thm3} follows naturally. 
%If $\sum_{i:d_i\leq\tau} [\gamma_i' - \zeta_i']>0$, then there exist some tasks that have not been assigned to any server. 
%In EDD-NR, a server that has just completed a task will be allocated to an unassigned task from the job with the earliest due time. Hence,
%$\sum_{i:d_i\leq\tau} [\gamma_i' - \zeta_i']=\sum_{i:d_i\leq\tau} [\gamma_i - \zeta_i] - 1 \leq \sum_{i:d_i\leq\tau} \xi_i -1 \leq \sum_{i:d_i\leq\tau} \xi_i'$.
%\end{proof}
%
%
%\begin{lemma}\label{lem_non_prmp2_thm3}
%Suppose that, under policy EDD-NR, $\{\bm{\gamma}',\bm{\zeta}'\}$ is obtained by adding a job with $b$ tasks and due time $d$ to the system whose state is $\{\bm{\gamma},\bm{\zeta}\}$. Further, suppose that, under policy $P'$, $\bm{\xi}'$ is obtained by adding a job with $b$ tasks and due time $d$ to the system whose state is $\bm{\xi}$.
%If
%\begin{eqnarray}
%\sum_{i:d_i\leq\tau} [\gamma_i- \zeta_i]\leq \sum_{i:d_i\leq\tau} \xi_i, ~\forall~\tau\in[0,\infty),\nonumber
%\end{eqnarray}
%then
%\begin{eqnarray}
%\sum_{i:d_i\leq\tau} [\gamma_i' - \zeta_i']\leq \sum_{i:d_i\leq\tau} \xi_i', ~\forall~\tau\in[0,\infty).\nonumber\end{eqnarray}
%\end{lemma}
%
%\begin{proof}
%If $d\leq\tau$, then
%$\sum_{i:d_i\leq\tau} [\gamma_i' - \zeta_i']\leq \sum_{i:d_i\leq\tau} [\gamma_i - \zeta_i] + b\leq \sum_{i:d_i\leq\tau} \xi_i+b \leq \sum_{i:d_i\leq\tau} \xi_i'$.
%
%If $d>\tau$, then
%$\sum_{i:d_i\leq\tau} [\gamma_i' - \zeta_i']\leq \sum_{i:d_i\leq\tau} [\gamma_i - \zeta_i] \leq \sum_{i:d_i\leq\tau} \xi_i \leq \sum_{i:d_i\leq\tau} \xi_i'$.
%\end{proof}
%
%Now we are ready to prove Lemma \ref{lemG4_thm3}.
%\ifreport
%\begin{proof}[Proof of Lemma \ref{lemG4_thm3}]
%\else
%\begin{proof}[of Lemma \ref{lemG4_thm3}]
%\fi
%Consider any busy period $[\tau,\nu)$ of policy $P'$. Then, in policy $P'$, all servers are busy during $[\tau,\nu)$, and are idle at time $\tau^-$ and time $\nu$. We prove \eqref{eq_lemG4_thm3} for $t\in[\tau,\nu)$ by considering two cases:
%
%\emph{Case 1: At time $t=\tau^-$, policy EDD-NR has $m$ tasks and the service of these tasks has just started.} Consider the system states of both policies at time $\tau^-$. The system state of policy EDD-NR satisfies 
%\begin{align}\label{proof_lemG4_1_thm3}
%\sum_{i=1}^n \gamma_i(\tau^-)= m, ~\bm{\gamma}(\tau^-)=\bm{\zeta}(\tau^-).
%\end{align}
%In policy $P'$, there is no task in the system at time $\tau^-$ such that 
%\begin{align}\label{proof_lemG4_5_thm3}
%\bm{\xi}(\tau^-)=\bm{0}. 
%\end{align}
%Consider the evolutions of both policies during $[\tau,\nu)$. 
%In policy $P'$, all servers are busy if there is at least one task. On the other hand, in policy EDD-NR, there is no task replication and all servers are busy if there are no less than $m$ tasks. 
%By \eqref{proof_lemG4_1_thm3} and \eqref{proof_lemG4_5_thm3}, it holds that for $t=\tau$
%\begin{align}\label{proof_lemG4_4_thm3}
%\sum_{i=1}^n \gamma_i(t)= \sum_{i=1}^n\xi_i(t) +m\geq m+1.
%\end{align}
%Therefore, the servers are all busy in policies $P'$ and policy EDD-NR at time $\tau$. By induction over time, we can show that for any sample path of policy $P'$, there is a sample path of policy EDD-NR with the same probability density such that \eqref{proof_lemG4_4_thm3} holds for all $t\in[\tau,\nu)$ and the task arrival times and task completion times of the two policies are exactly the same  during $[\tau,\nu)$. Using Lemma \ref{lem_non_prmp1_thm3}, Lemma \ref{lem_non_prmp2_thm3}, and the initial states at time $\tau^-$, we can prove that \eqref{eq_lemG4_thm3} holds for all $t\in[\tau,\nu)$ on these two sample paths.
%
%\emph{Case 2: At time $t=\tau^-$, policy EDD-NR has less than $m$ tasks or the service of these tasks started before time $\tau^-$}. In both \emph{Case 1} and \emph{Case 2}, the sample path evolutions of policy $P'$ are the same. On the other hand, in policy EDD-NR, the tasks are completed earlier in \emph{Case 2} than in \emph{Case 1}. Therefore, \eqref{eq_lemG4_thm3}  also holds in \emph{Case 2} for $t\in[\tau,\nu)$.
%
%%Note that the case that policy EDD-NR has more than $m$ tasks at time $\tau^-$ will not happen. This will be clear 
%Let $[\tau_1,\nu_1)$ be the next busy period of policy $P'$ with $\nu<\tau_1$. Then, $[\nu,\tau_1)$ is an idle period of policy $P'$. We now prove \eqref{eq_lemG4_thm3} during the idle period $[\nu,\tau_1)$. 
%Because all servers are idle during $[\nu,\tau_1)$ in policy $P'$, it follows that 
%\begin{align}\label{proof_lemG4_2_thm3}
%\bm{\xi}(t)=\bm{0},~t\in[\nu,\tau_1).
%\end{align}
%Hence, there is no task arrival during $[\nu,\tau_1)$; otherwise, \eqref{proof_lemG4_2_thm3} cannot be true.
%On the other hand, at time $\nu$ there are no more than $m$ tasks in policy EDD-NR such that 
%\begin{align}
%\bm{\gamma}(\nu)=\bm{\zeta}(\nu).\nonumber
%\end{align}
%Because there is no task arrival during $[\nu,\tau_1)$, policy EDD-NR satisfies
%\begin{align}\label{proof_lemG4_3_thm3}
%\bm{\gamma}(t)=\bm{\zeta}(t),~t\in[\nu,\tau_1).
%\end{align}
%By \eqref{proof_lemG4_2_thm3} and \eqref{proof_lemG4_3_thm3}, \eqref{eq_lemG4_thm3} holds during $[\nu,\tau_1)$.
%Further, from \eqref{proof_lemG4_3_thm3}, we can obtain
%\begin{align}
%\sum_{i=1}^n \gamma_i(\tau_1^-)=\sum_{i=1}^n \zeta_i(\tau_1^-)\leq m,
%\end{align}
%such that there are no more than $m$ tasks at time $t=\tau_1^-$ in policy EDD-NR. Hence, either \emph{Case 1} or \emph{Case 2} is satisfied at time $t=\tau_1^-$. Then, we can use the above arguments to prove that  \eqref{eq_lemG4_thm3} holds during the next busy period $[\tau_1,\nu_1)$ of policy $P'$.
%
%
%Finally, by taking an induction over the busy and idle periods of policy $P'$,  Lemma \ref{lemG4_thm3} is proven.
%\end{proof}
%
%
%\ifreport
%\begin{proof}[Proof of Condition 3]
%\else
%\begin{proof}[of Condition 3]
%\fi
%%Let the evolution of the system state under some scheduling policy be on a space $(\Omega,\mathcal{F},P)$. Each $\omega\in\Omega$ corresponds to a sample path of policy $P'$ and a sample path of policy EDD-NR. The job arrival parameters $\mathcal{I}$ is fixed for all $\omega\in\Omega$. 
%%Let $(C_{w_1}(P'),\ldots,c_{N:N}(P'))$ be a permute of the job completion time sequence $(c_{1}(P'),\ldots,c_{N}(P'))$ in the increasing order, such that $c_{i:N}(P')\leq c_{i+1:N}(P')$. 
%
%%Pick any $\omega\in\Omega$ and consider the first job completion time $C_{w_1}(P')$ of policy $P'$. Suppose that there are $y$ job arrivals during $[0,C_{w_1}(P'))$. 
%
%We  prove Condition 3 by induction. Consider the sample paths of policy $P'$ and policy EDD-NR satisfying Lemma \ref{lemG4_thm3}. Suppose that job $w_i$ is the $i$-th completed job in the sample path of policy $P'$. We first show that 
%\begin{align}\label{eq_Condition_3_1_thm3}
%U_{w_1}(\text{EDD-NR}) \leq C_{w_1}(P').
%\end{align}
%
%According to the construction of policy $P'$, at time $t=C_{w_1}(P')$, the system state of policy $P'$ must satisfy 
%\begin{align}\label{eq_proof_0_thm3}
%\sum_{i:d_i\leq d_{w_1}}\xi_i(C_{w_1}(P'))=0.
%\end{align}
%That is, when job $w_1$ leaves the system in policy $P'$, no job with a due time earlier than $d_{w_1}$ can exist in the system.
%This and Lemma \ref{lemG4_thm3} imply
%%Hence, there are $y-1$ unfinished jobs at time $C_{w_1}(P')$ such that
%%Invoking Lemma \ref{lemG4}, we can obtain
%\begin{align}\label{eq_proof_1_thm3}
%\sum_{i:d_i\leq d_{w_1}} \gamma_i(C_{w_1}(P'))\leq \sum_{i:d_i\leq d_{w_1}}  \zeta_i(C_{w_1}(P')).
%\end{align}
%
%
%
%By \emph{Definition \ref{def_state_thm3}}, we have $\gamma_i(t)\geq \zeta_i(t)$. Hence, the system state of policy EDD-NR satisfies 
%\begin{align}\label{eq_proof_2_thm3}
%\!\!\gamma_i(C_{w_1}(P'))= \zeta_i(C_{w_1}(P')),
%\end{align}
%for all job $i$ with $d_i\leq d_{w_1}$. In particular, job $w_1$ satisfy
%\begin{align}\label{eq_proof_3_thm3}
%\gamma_{w_1}(C_{w_1}(P'))= \zeta_{w_1}(C_{w_1}(P')).
%\end{align}
%This tells us that in EDD-NR, all tasks of job $w_1$ are either completed or under service at time $C_{w_1}(P')$. Hence, \eqref{eq_Condition_3_1_thm3} is proven.
%%\begin{align}%\label{eq_proof_9}
%%U_{w_1}(\text{EDD-NR}) \leq C_{w_1}(P'),\nonumber
%%\end{align}
%%which implies \eqref{eq_Condition_3_1}.
%
%Next, we prove the induction step. Suppose that 
%\begin{align}
%U_{w_i}(\text{EDD-NR}) \leq C_{w_i}(P'),~i=1,\ldots,j,\nonumber
%\end{align}
%we will show that \begin{align}\label{eq_proof_9_thm3}
%U_{w_{j+1}}(\text{EDD-NR}) \leq C_{w_{j+1}}(P').
%\end{align}
%At time $t=C_{w_{j+1}}(P')$, the system state of policy $P'$ satisfies 
%\begin{align}
%\sum_{i: d_i\leq d_{w_{j+1}}}\xi_i(C_{w_{j+1}}(P'))=0.\nonumber
%\end{align}
%That is, when job $w_{j+1}$ leaves the system in policy $P'$, no job with a due time earlier than $d_{w_{j+1}}$ can exist in the system.
%Then, by following the arguments of \eqref{eq_proof_1_thm3}-\eqref{eq_proof_3_thm3}, we can obtain that job $w_{j+1}$ satisfies
%\begin{align}\label{eq_proof_4_thm3}
%\gamma_{w_{j+1}}(C_{w_{j+1}}(P'))= \zeta_{w_{j+1}}(C_{w_{j+1}}(P')).
%\end{align}
%Then, \eqref{eq_proof_4_thm3} tells us that in EDD-NR, all tasks of job $w_{j+1}$ are either completed or under service at time $t=C_{w_{j+1}}(P')$. Hence, \eqref{eq_proof_9_thm3} is proven.
%
%By induction, we can obtain
%\begin{align}\label{eq_proof_10_thm3}
%U_{i}(\text{EDD-NR}) \leq C_{i}(P'),~i=1,\ldots,n.
%\end{align}
%Consider all possible sample paths of policy $P'$ and policy EDD-NR, the stochastic ordering result in \eqref{eq_condition3_thm3} follows.
%\end{proof}
%After establishing conditions 1-3 of Thoerem \ref{lem2} for policy EDD-NR,  we can prove \eqref{eq_delaygap1_thm3}. 
%
%Similar proof procedure can be used to prove \eqref{eq_delaygap2_thm3}. By this, Theorem \ref{thm3} is proven.
%\subsection{Proof of Corollary~\ref{coro_thm3_1}} \label{sec_app_3_2} 
%Because conditions 1-3 of Thoerem \ref{lem2} have been established in Appendix \ref{sec_app_3_1},  Corollary~\ref{coro_thm3_1} directly follows from Corollary \ref{coro2}.
