# Supplementary material for: Near Delay-Optimal Scheduling of Batch Jobs in Multi-Server Systems
Source: arXiv:2309.16880 source file (2023-09-28)
Supplement: Supplementary file 20 [file appendices_dis.tex]

% !TEX root = ./replication.tex
%\section{Proofs of Thoerem~10 and Corollary 10} \label{app_dis_EDD}
%Similar with the proof of Theorem \ref{thm2}, we can show that policy FCFS-R is more work-efficient than any policy $\pi\in\Pi$. Then, Theorem \ref{thm6} follows from Thoerem \ref{lem3}, and Corollary \ref{coro6_1} follows from Corollary \ref{coro3_1}.
